# Supplementary material for: Amplitude maximization in stable systems, Schur positivity, and some conjectures on polynomial interpolation
Source: arXiv:2508.13554 source file (2025-08-20)
Supplement: Supplementary file 1 [file appendix.tex]

%\section{Deferred proofs}
%\label{apx:deferred-proofs}

\section{Auxiliary results}
\label{apx:aux}

\subsection{Bounding the norm of a convolution power}
\label{apx:convolution-powers}

%Proof of Proposition~\ref{prop:convolution-powers} for nondyadic powers

\begin{proposition}[Convolution powers]
\label{prop:convolution-powers}
If~$X \subseteq \C(\Z)$ admits a reproducing filter~$\phi \in  \C_m(\Z)$ with~$\| \phi \|_2 \le \frac{\sR}{\sqrt{2m+1}}$, then
for any~$k \in \{2,3,...\}$,~$\phi^{k} \in \C_{km}(\Z)$ is also reproducing for~$X$, with
\[
\|\phi^{k}\|_2 \le \|\F_{km} [\phi^{k}]\|_1 \le \frac{c_k \sR^k}{\sqrt{2km+1}}
\]
where~$c_{k} = 2^{k-1}$ for~$k = 2^p$ and~$c_{2k+1} \le 3 \sqrt{2k+1}c_k^2$ for~$k \in \N$; as such,~$\log(c_k) = O(k\log k)$.
\end{proposition}
\begin{proof}
%The case~$k = 2$ corresponds to Proposition~\ref{prop:convolution}. 
%C~$k = 2$ is proved.
The reproducing property follows from~$1-\phi^k(z) = (1-\phi(z))(1+\phi(z)+...+\phi^{k-1}(z))$.
\iffalse
For~$k = 3$, 
\[
\begin{aligned}
\|\F_{3m} [\phi^{3}]\|_1 
%\stackrel{\eqref{def:DFT}}{=}  \frac{1}{\sqrt{6m+1}} \sum_{z \in \T_{3m}} \left| \phi^3(z) \right|
%&\le \frac{1}{\sqrt{6m+1}} \max_{\zeta \in \T_{3m}} \left| \phi(\zeta) \right| \sum_{z \in \T_{3m}} \left| \phi^2(z) \right| \\
%&=(6m+1) \; \|\F_{3m}[\phi]\|_{\infty} \, \|\F_{3m}[\phi]\|_{2}^2
\stackrel{\eqref{def:DFT}}{=} 
	(6m+1) \, \|\F_{3m}[\phi]\|_{3}^3
\le
	(6m+1) \, \|\F_{3m}[\phi]\|_{2}^3
=
	(6m+1) \, \|\phi\|_{2}^3	
\le \frac{3 \sR^3}{\sqrt{2m+1}}.
%\le \frac{3\sqrt{3} \sR^3}{\sqrt{6m+1}}.
\end{aligned}
\]
\fi
For~$k = 2^p$, we proceed by induction over~$p$: assume that~$\|\phi^{k}\|_2 \le \|\F_{km} [\phi^{k}]\|_1 \le \frac{c_{k} \sR^{k}}{\sqrt{2km+1}}$, then
%mimicking the case of Proposition~\ref{prop:convolution},
%and define~$p(k) := \frac{k+1}{k}$. \[
\[
\begin{aligned}
\|\F_{2km} [\phi^{2k}]\|_1 
\stackrel{\eqref{def:DFT}}{=}  
\sqrt{4km+1} \|\F_{2km}[\phi^k] \|_2^2 
= \sqrt{4km+1} \|\phi^k\|_2^2 
\le
\frac{\sqrt{4km+1}\,c_{k}^2 \sR^{2k}}{2km+1}
\le 
\frac{2c_{k}^2 \sR^{2k}}{\sqrt{4km+1}}.
\end{aligned}
\]
Whence~$c_{2k}^{\vphantom 2} = 2c_{k}^2$ for all~$k \in \N$. 
Unrolling this recursion we arrive at~$c_{2^p} = 2^{\sum_{j = 0}^{p-1} 2^j} = 2^{2^p-1}$.
%Our bound for nondyadic powers~$k \ne 2^p$ is crude; we include its proof in the appendix.
Now, to bound~$c_{2k+1}$ in terms of~$c_{k}$ observe that
%\paragraph{Case $k = 2p+1$.}
%In this case,
\[
\begin{aligned}
\|\F_{(2k+1)m} [\phi^{k}]\|_1 
&\stackrel{\eqref{def:DFT}}{=}  
\frac{1}{\sqrt{2(2k+1)m+1}} \sum_{z \in \T_{(2k+1)m}} \left| \phi^{2k+1}(z) \right| \\
&\le
(2(2k+1)m+1)\,\| \F_{(2k+1)m}[\phi] \|_{\infty} \|\F_{(2k+1)m}[\phi^k] \|_2^2 \\
&\le 
(2(2k+1)m+1)\,\| \phi\|_2^{\vphantom 2} \,\|\phi^k\|_2^2 \\
&\le 
\frac{2(2k+1)m+1}{2km+1} \, \frac{c_{k}^2 \sR^{2k+1}}{\sqrt{2m+1}} \\
&\le 
\frac{2k+1}{k} \, \frac{c_{k}^2 \sR^{2k+1}}{\sqrt{2m+1}} 
\le 
\frac{3\sqrt{2k+1}c_{k}^2 \sR^{2k+1}}{\sqrt{2(2k+1)m+1}}.
\end{aligned}
\]
%where we used that~$\frac{2k+1}{k} \le 3$ for~$k \in \N$.
As such,~$c_{2k+1}^{\vphantom 2} \le 3\sqrt{2k+1} c_{k}^2$, indeed.
Finally, to verify that~$\log(c_k) = O(k \log k)$ for all~$k \ge 2$, it suffices to consider the binary representation of~$k$, and alternate between the two cases.
\end{proof}

%\section{Trigonometric interpolation over equidistant grids}
%\label{apx:trig-interpol}

\subsection{Extreme points of the ball of the norm~$\max\{\|\cdot\|_1, s\|\cdot\|_\infty\}$ on~$\C^n$}
\label{apx:extreme-points}
In what follows, we let~$n,s \in \N \cup \{0\}$ and define the sets~$\Comp^n(s), \Real^n(s), \Posi^{n}(s)$ as follows:
\begin{equation}
\label{def:cap-balls}
\bald
\Comp^n(s)
	&:= \{w \in \C^{n}: \;  \| w \|_{\infty} \le 1, \, \|w\|_1 \le s\}, \\
\Real^n(s)
	&:= \{u \in \R^{n}: \;  \| u \|_{\infty} \le 1, \, \|u\|_1 \le s\}, \\
\Posi^{n}(s)
	&:= \{u \in \R_+^{n}: \;  \| u \|_{\infty} \le 1, \, \|u\|_1 \le s\}.
%\Over(n,p,s)
%	&:= \{\vphi \in \C_n(\Z): \F_{n+p}[\vphi] \in \Comp(2n+2p+1,s)\}.
\eald
\end{equation}
%The geometry of the set~$\Real(n,k)$ has been thoroughly studied in~\cite{deza2021polytopal}; in particular,
We first recall the (known) explicit characterizations of the vertices of~$\Posi^n(s)$ and~$\Real^n(s)$.
\begin{proposition}[{\cite[Thm.~2.1 and Eq.~(2.1)]{deza2021polytopal}}]
\label{prop:cap-real}
The polytope~$\Posi^n(s)$ (resp.~$\Real^n(s)$) has~${n \choose s}$ $ $  $ $(resp.~$2^s {n \choose s}$) vertices, namely all~$s$-sparse vectors with entries in~$\{0,1\}$ (resp.~$\{-1, 0, 1\}$). 
\end{proposition}
As an immediate corollary, we restrict the possible structure of extremal points for~$\Comp^n(s)$. 
\begin{proposition}
\label{prop:cap-comp}
Let~$e^{0}, ..., e^{n-1}$ be the canonical basis of~$\R^{n}$.
Any extremal point of~$\Comp^n(s)$ is of the form~$\sum_{j = 0}^{n-1} z_j u_j e^j$ for some~$z_0, ..., z_{n-1} \in \T$ and~$s$-sparse binary vector~$u = (u_0,...,u_{n-1})$.
\end{proposition}
\begin{proof}
Let~$w \in \Comp^n(s)$, then~$|w| \in \Posi^n(s)$ for~$|w| = (|w_0|, ..., |w_{n-1}|)$.
By Proposition~\ref{prop:cap-real}, there exist a sequence~$u^{1}, u^{2}, ...$ of~$s$-sparse binary vectors and a sequence~$\alpha_1, \alpha_2, ...$ of nonnegative coefficients adding up to 1, such that
%~$|w|$ is a convex combination of~$s$-sparse vectors with unit nonzero entries. In other words,
%\begin{equation}
%\label{eq:convex-combination-posi}
$
|w_j| = \sum_{k} \alpha_k (u^{k})_j
$
%\quad j \in \{0,..., n\}
%\end{equation}
for~$0 \le j \le n-1$. Multiplying this by~$z_j := w_j / |w_j| \in \T$ we get
%Multiplying~\eqref{eq:convex-combination-posi} 
%\begin{equation}
%\label{eq:convex-combination-comp}
$w_j = \sum_{k} \alpha_k z_j (u^{k})_j$ 
%\quad j \in \{0,..., n\}.
%\end{equation}
for~$0 \le j \le n-1$.
In other words, any~$w \in \Comp^n(s)$ is a convex combination of vectors of the form~$( z_0 u_0, ..., z_{n-1} u_{n-1})$, where each~$u = (u_0, ..., u_{n-1})$ is an~$s$-sparse binary vector.
\end{proof}

\section{Technical results on trigonometric interpolation}
\label{apx:dirichlet-and-fejer}

\subsection{Dirichlet and Fej\'er kernels}

The Dirichlet and Fej\'er kernels, respectively, are the following Laurent polynomials~\cite{zygmund2002trigonometric}:
\begin{align}
\label{def:Dir-and-Fej}
\Dir_m(z) := \sum_{|k| \le m} z^k, \quad
\Fej_m(z) 
&:= \sum_{|k| \le m} \left(1-\frac{|k|}{m+1}\right)z^k.
%= \frac{1}{2n+1} \left|\sum_{k=0}^{2n} z^k \right|.
%= \frac{1}{2n+1}\Dir_n(z)^2.
\end{align}
That is,~$\Dir_m(z)$ is the~$z$-transform of the rectangular window signal~$u_t = \ones\{|t| \le m\}$;~$\Fej_{m}(z)$ that of the triangular window signal~$v_t (1-\frac{|t|}{m+1}) \ones\{|t| \le m\}$, 
and~$\Fej_{2m}(z) = \frac{1}{4m+1} \Dir_m^2(z)$.
Note that~$\frac{1}{2m+1}\Dir_m(1) = \frac{1}{m+1}\Fej_m(1) = 1$. 
%as~$m \to \infty$,~$\tfrac{1}{2m+1} \Dir_m(z) \to 0$, $\tfrac{1}{m+1} \Fej_m(z) \to 0$ for~$z \ne 1$.
These kernels can be recast as trigonometric polynomials:
\[
\dir_m(\omega) := \Dir_m(e^{i\omega}) = \frac{\sin((2m+1)\frac{\omega}{2})}{\sin(\frac{\omega}{2})},
\quad
\fej_m(\omega) := \Fej_m(e^{i\omega}) = \frac{1}{m+1} \left(\frac{1-\cos((m+1)\omega)}{1-\cos(\omega)} \right).
\]
%the normalization in~\eqref{def:Dir} and~\eqref{def:Fej} is such that~$\dir_n(0) = \fej_n(0) = 1$.
Finally, we define the causal counterpart of the Fej\'er kernel by appropriately shifting~$\Fej_m(z)$:
\begin{equation}
\label{def:Fej-causal}
\Fej_{2m}^+(z) := z^m \Fej_m(z).
\end{equation}
Note that~$\Fej_{2m}^+ \in \C_{2m}^+(\Z)$. Moreover,~$\Fej_{2m}^+(1) = m+1$, and~$|\Fej_{2m}^+(z)| = |\Fej_m(z)|$ for all~$z \in \T$.
%we define the linearly decreasing kernel -- the one-sided counterpart of the Fej\'er kernel:
%\begin{equation}
%\label{def:Fej-causal}
%%\Dir_m^+(z) := \sum_{k = 0}^m z^k, \quad
%\Fej_m^+(z) := \sum_{k = 0}^m \left(1-\frac{k}{m+1}\right)z^k.
%%= \frac{1}{2n+1} \left|\sum_{k=0}^{2n} z^k \right|.
%%= \frac{1}{2n+1}\Dir_n(z)^2.
%\end{equation}
%Its properties can be easily inferred from those of~$\Fej_m(z)$, since~$\Fej_m(z) = \Fej_m^+(z) + \Fej_m^+(z^{-1}) - 1$.
%In particular,~$\Fej_m^+(1) = \frac{1}{2}(\Fej_m(1) + 1) = \frac{m+2}{2}$, which suggests~$\frac{2}{m+2}$ as the normalization factor.

\paragraph{Summation over equidistant grids.}
We bound the sums of~$|\Dir_n^{\vphantom+}|$,~$|\Fej_n^{\vphantom+}|$,~$|\Fej_{2n}^+|$ over~$\T_N$.
%We have the following estimates for the sums of~$|\Dir_n|$,~$|\Fej_n|$.
\begin{lemma}
\label{lem:oversampling}
For any~$n,N \in \N$ and~$a \in \T$, letting~$H_N$ be the~$N^{\textup{th}}$ harmonic number, one has
\[
\begin{aligned}
\frac{1}{2N+1}\sum_{w \in \T_N} \left|\Dir_{n}\Big(\frac{w}{a}\Big)\right|
&\le \frac{4n+2}{2N+1} + H_N,\\
%\quad\text{and}\quad
\frac{1}{2N+1}\sum_{w \in \T_N} \left|\Fej_{2n}^+\Big(\frac{w}{a}\Big)\right|
= \frac{1}{2N+1}\sum_{w \in \T_N} \left|\Fej_{n}\Big(\frac{w}{a}\Big)\right|
&\le \frac{2n+2}{2N+1} + \left( \frac{2N+1}{2n+2} \right) \frac{\pi^2}{6}.
\end{aligned}
\]
\end{lemma}
\begin{proof}
Since~$|\Fej_{2n}(z)| = |\Fej_n^+(z)|$ for~$z \in \T$, the summation of~$|\Fej_{2n}^+|$ reduces to that of~$|\Fej_{n}|$. 
Now, for any~$a \in \C$, at most 2 points of the grid~$\{\frac{w}{a}: w \in \T_N\}$ have argument in~$(-\frac{2\pi}{2N+1},\frac{2\pi}{2N+1})$.
Each of them contributes at most~$\Dir_n(1) = 2n+1$ or~$\Fej_n(1) = n+1$ to the respective sum. 
As for the remaining points, we use the following elementary estimates valid for all~$\omega \in [-\pi,\pi]$,
\vspace{-0.1cm}\[
|\dir_n(\omega)| \le \frac{1}{|\sin(\frac{\omega}{2})|} \le \frac{\pi}{|\omega|}
\quad\text{and}\quad
0 \le (n+1)\fej_n(\omega) \le \frac{1}{\sin^2(\frac{\omega}{2})} \le \frac{\pi^2}{\omega^2},
\]
whose right-hand sides decrease in~$|\omega|$, and summate separately over at most~$N$ points with argument in~$[\frac{2\pi}{2N+1}, \pi]$ and at most~$N$ points with argument in~$[-\pi,-\frac{2\pi}{2N+1}]$. 
Overall, this gives
\[
\begin{aligned}
\sum_{w \in \T_N} \left|\Dir_{n} \hspace{-0.1cm}\left(\frac{w}{a}\right)\right|
&\le 2\left(2n+1 + \sum_{k = 1}^N \frac{\pi}{\arg(\chi_{k,N})} \hspace{-0.1cm}\right)
= {4n+2} + (2N+1)\sum_{k = 1}^N \frac{1}{k},\\
\sum_{w \in \T_N} \left|\Fej_{n}\hspace{-0.1cm}\left(\frac{w}{a}\right)\right|
&\le 2\left(n+1 +  \frac{1}{n+1} \sum_{k = 1}^N \frac{\pi^2}{\arg(\chi_{k,N})^2} \hspace{-0.1cm}\right) 
= {2n+2} + \frac{(2N+1)^2}{2n+2} \sum_{k = 1}^N \frac{1}{k^2}.
\end{aligned}
\]
Here we used that~$\arg(\chi_{k,N}) = \frac{2\pi k}{2N+1}$ for~$k \in \{1,...,N\}$;~cf.~\eqref{def:DFT-grid}. 
\end{proof}

\paragraph{Oversampling bounds.} 
%\subsection{Oversampling bounds}
%\label{apx:oversampling}
As it was observed in~\cite{harchaoui2019adaptive}, the Dirichlet kernel summation estimate of Lemma~\ref{lem:oversampling} directly implies a uniform estimate for the inflation of~$\ell_1$-norm with oversampling, that is~the uniform over~$\vphi \in \C_n(\Z)$ upper bound for the ratio~$\|\F_{N}[\vphi]\|_{1}/\|\F_{n}[\vphi]\|_{1}$ with~$N \ge n$. 
%Let us remind it.
%(For~$p = 2$, there is no change due to Parseval's identity.)
%For~$\ell_1$-norm, this is controlled by the Dirichlet kernel. 
%Namely, from the proof of~\cite[Lem.~2]{harchaoui2019adaptive} we extract the following result.

\begin{lemma}[Oversampling in~$\ell_1$]
\label{lem:oversampling-l1}
For any~$n,N \in \N$ such that~$N \ge n$, and nonzero~$\vphi \in \C_n(\Z)$,
\[
\begin{aligned}
\frac{\| \F_{N}[\vphi] \|_1}{ \| \F_{n}[\vphi] \|_1} 
&\le \frac{1}{\sqrt{(2N+1)(2n+1)}} \max_{a \in \T_n} \sum_{w \in \T_{N}} \left|\Dir_{n}\left(\frac{w}{a}\right)\right| 
\le \sqrt{\frac{2N+1}{2n+1}} \log(eN) + 2\sqrt{\frac{2n+1}{2N+1}}.
\end{aligned}
\]
\begin{proof}
We first note that the convex function~$\| \F_{N}^{\vphantom{\,-1}}[\F_{n}^{\,-1}[\cdot]]\|_1$ is maximized at an extreme point of the unit~$\ell_1$-ball in~$\C^{2n+1}$, i.e.~on a vector of the form
$
z e^{j},
$
where~$z \in \T$ and~$e^{j}$,~$0 \le j \le 2n$, is the~$j^\textup{th}$ canonical basis vector of~$\R^{2n+1}$. 
As the result,
%This leads to the identity
\[
\bald
\max_{\vphi \in \C_n(\Z) \setminus 0} \frac{\| \F_{N}[\vphi] \|_1}{ \| \F_{n}[\vphi] \|_1} 
%&=  \max_{0 \le j \le 2n, \; z \in \T} \| \F_{N}^{\vphantom{\pinv}}[\F_n^\pinv[ze^j]] \|_1  
&=  \max_{0 \le j \le 2n} \| \F_{N}^{\vphantom{\,-1}}[\F_n^{\,-1}[e^j]] \|_1 
= \frac{1}{\sqrt{(2N+1)(2n+1)}} \max_{0 \le j \le 2n} \sum_{k = 0}^{2N} \left|\Dir_{n}\left(\frac{\chi_{k,N}}{\chi_{j,n}}\right)\right|.
\eald
\]
After that, it only remains to invoke Lemma~\ref{lem:oversampling}. 
\end{proof}
\end{lemma}
\begin{remark}
\label{rem:dirichlet-log}
{\em For~$N \ge (1+c)n$, the inequality of Lemma~\ref{lem:oversampling-l1} is sharp up to a constant factor.}
\end{remark}
Below we give a counterpart result for~$\ell_\infty$-norm. 
In the context of trigonometric interpolation, the corresponding ratio is known as the Lebesgue constant, and a sharp estimate is known for it (e.g.~\cite{ehlich1966auswertung},~\cite[Thm.~2.1]{sorevik2016trigonometric}).
We give a standalone estimate to keep the paper self-contained.
%(Besides, our bounds in Lemma~\ref{lem:oracle-norm-bounds} allow for~$a \ne 1$.)

\begin{lemma}[Oversampling in~$\ell_\infty$]
\label{lem:oversampling-linf}
For any~$n,N \in \N$ with~$N \ge n$, and nonzero~$\vphi \in \C_n(\Z)$, 
\[
\begin{aligned}
\frac{\| \F_{N}[\vphi] \|_\infty}{ \| \F_{n}[\vphi] \|_\infty} 
\le 
	\frac{1}{\sqrt{(2N+1)(2n+1)}} \max_{a \in \T_N} \sum_{w \in \T_n} \left| \Dir_{n} \left( \frac{w}{a} \right) \right|
	\le \sqrt{\frac{2n+1}{2N+1}} (H_n + 2).
\end{aligned}
\]
As a consequence, for any~$\vphi \in \C_n(\Z)$ it holds that\,~$\max_{z \in \T} |\vphi(z)| \le (H_n + 2) \, \max_{z \in \T_n} |\vphi(z)|$.
\end{lemma}
\begin{proof}
The convex function~$\| \F_{N}^{\vphantom{\,-1}}[\F_{n}^{\,-1}[\cdot]]\|_\infty$ is maximized at an extreme point of the unit~$\ell_\infty$-ball in~$\C^{2n+1}$, i.e.~on a vector of the form~$(z_0, z_1, ..., z_{2n})$
%$
%\sum_{j = 0}^{2n} z_j e^{j}
%$
where~$z_j \in \T$ for~$0 \le j \le 2n$.
%and~$e^{j}$ is the~$j^\textup{th}$ canonical basis vector of~$\R^{2n+1}$. 
As the result,
\[
\bald
\max_{\vphi \in \C_n(\Z) \setminus 0} \frac{\| \F_{N}[\vphi] \|_\infty}{ \| \F_{n}[\vphi] \|_\infty} 
&=  
	\max_{z_0, ..., z_{2n} \in \T} \big\| \F_{N}^{\vphantom{\,-1}} \big[\F_n^{\,-1} \big[ z_0 e^0 + z_1 e^1 + ... + z_{2n} e^{2n} \big] \big] \big\|_\infty \\
&= 
	\frac{1}{\sqrt{(2N+1)(2n+1)}} \max_{z_0, ..., z_{2n} \in \T} \max_{0 \le k \le 2N} \left| \sum_{j = 0}^{2n} z_j\Dir_{n} \left( \frac{\chi_{j,n}}{\chi_{k,N}} \right) \right| \\
&= 
	\frac{1}{\sqrt{(2N+1)(2n+1)}} \max_{0 \le k \le 2N} \sum_{j = 0}^{2n} \left| \Dir_{n} \left( \frac{\chi_{j,n}}{\chi_{k,N}} \right) \right|.
\eald
\]
As previously, we conclude by invoking Lemma~\ref{lem:oversampling}. 
\end{proof}

We are now about to enhance the previous result: it turns out that the worst-case ratio of~$\ell_\infty$-norms reduces to~$O(\log(s))$ if we only allow for~$s$-sparse vectors in the spectral domain.

\begin{lemma}[Oversampling in~$\ell_\infty$ under sparsity]
\label{lem:oversampling-linf-sparse}
For~$s,n,N \in \N$ such that~$N \ge n$, one has
\[
\bald
\max_{w \in \Comp^{2n+1}(s)} \| \F_{N}^{\vphantom{\,-1}}[\F_n^{\,-1}[w]] \|_\infty
\le \sqrt{\frac{2n+1}{2N+1}} (\log(\lceil s/2 \rceil) + 3).
\eald
\]
%Equivalently,~$\vphi = \F_n^\pinv[w]$ satisfies~$\max_{z \in \T} |\vphi(z)| \le (H_s + 3) \max_{z \in \T_n} |\vphi(z)|$ for all~$w \in \Comp^{2n+1}(s)$.
\end{lemma}

\begin{proof}

We can assume that~$s \le 2n$, as otherwise the claim reduces to Lemma~\ref{lem:oversampling-linf}. 
The convex function~$\| \F_{N}^{\vphantom{\,-1}}[\F_{n}^{\,-1}[\cdot]]\|_\infty$ is maximized at an extreme point of~$\Comp^{2n+1}(s)$. By Proposition~\ref{prop:cap-comp}, these are of the form~$z_1 e^{j_1} + ... z_s e^{j_s}$ for some~$z_1, ..., z_s \in \T$ and~$\{j_1, ...,  j_s\} \subset \{0, 1, ..., 2n\}$. 
Thus,
\[
\begin{aligned}
&\max_{w \in \Comp^{2n+1}(s)} \| \F_{N}^{\vphantom{\,-1}}[\F_n^{\,-1}[w]] \|_\infty
=  
	\max_{
	\scriptsize
	\begin{aligned}
		\{j_1, ...,  j_s\} &\subset \{0, 1, ..., 2n\},\\
		z_1, ..., z_{s}    &\in \T
	\end{aligned}
	} \; \big\| \F_{N}^{\vphantom{\,-1}} \big[\F_n^{\,-1} \big[ z_1 e^{j_1} + ... + z_{s} e^{j_s} \big] \big] \big\|_\infty \\
&= 
	\frac{1}{\sqrt{(2N+1)(2n+1)}} 
	\max_{
	\scriptsize
	\begin{aligned}
		\{j_1, ...,  j_s\} &\subset \{0, 1, ..., 2n\},\\
		z_1, ..., z_{s}    &\in \T
	\end{aligned}
	} \; \max_{0 \le k \le 2N} \left| z_1 \Dir_{n} \hspace{-0.1cm}\left( \frac{\chi_{j_1,n}}{\chi_{k,N}} \right) + ... + z_s \Dir_{n} \hspace{-0.1cm}\left( \frac{\chi_{j_s,n}}{\chi_{k,N}} \right)\right| \\
&= 
	\frac{1}{\sqrt{(2N+1)(2n+1)}} 
	\max_{\{j_1, ...,  j_s\} \subset \{0, 1, ..., 2n\}} \,  \max_{0 \le k \le 2N} \left( \left| \Dir_{n} \hspace{-0.1cm}\left( \frac{\chi_{j_1,n}}{\chi_{k,N}} \right) \right| + ... + \left| \Dir_{n} \hspace{-0.1cm}\left( \frac{\chi_{j_s,n}}{\chi_{k,N}} \right) \right| \right) \\
&\le 
\hspace{-0.05cm}\sqrt{\frac{2n+1}{2N+1}} (H_{\lceil s/2 \rceil} + 2).
\end{aligned}
\]
In the end, we proceeded as in the proof of Lemma~\ref{lem:oversampling} using the bound~$|\dir_n(\omega)| \le {\pi}{|\omega|^{-1}}$.
\end{proof}

\section{Technical results concerning shift-invariant subspaces of~$\C(\Z)$}
\label{apx:shift-inv}

\subsection{Characterization of finite-dimensional shift-invariant subspaces of~$\C(\Z)$}
\label{sec:SIS-characterization}

As shown in~\cite{harchaoui2019adaptive},~$s$-dimensional shift-invariant subspaces of~$\C(\Z)$ can be characterized in terms of the corresponding characteristic polynomial.\footnote{Characterization of the invariant subspaces for the restriction of~$\Delta$ to~$\ell^2$ is a classical topic~\cite{beurling1949two,halmos1961shifts,nikol'skii1967invariant}. Yet, these classical results seem to be limited to Hilbert spaces, and therefore not allowing to recover Proposition~\ref{prop:SIS-characterization}.}
To state the corresponding result, we start with a brief reminder.
The {\em lag} operator~$\Delta: \C(\Z) \to \C(\Z)$ is defined by~$(\Delta x)_t = x_{t-1}$.
%In the canonical basis of~$\C(\Z)$ consisting of lagged unit impulse signals~$\{ e^{\tau}\}_{\tau \in \Z}$,~$\Delta$ is represented by the infinite matrix that has~$1$ in the first diagonal above the main diagonal, and~$0$ elsewhere. 
A linear subspace~$X$ of~$\C(\Z)$ is called {\em shift-invariant} if it is an invariant subspace of~$\Delta$, that is~$\Delta X \subseteq X$.
An easy exercise is to verify that~$\Delta$ is bijective on any shift-invariant subspace, thus~$\Delta X = X$.
%The next result gives full characterization of shift-invariant subspaces of~$\C(\Z)$.
%The difficulty when adapting this classical machinery to our situation is that~$\C(\Z)$ is not a Hilbert space. 
%As such, Corollary~\ref{cor:commutation} below might be a known result; yet, we did not manage to find any specific reference.
%In order to present it, let us recall some definitions.
\begin{proposition}[{\cite[Proposition~5]{harchaoui2019adaptive}}]
\label{prop:SIS-characterization} 
%The set of solutions of a homogeneous linear difference equation~$(p(\Delta)[x])_t \equiv 0$ 
%with a characteristic polynomial $p(z) = 1 + p_1 z + ... + p_s z^s$ of degree~$s$ is a shift-invariant subspace of dimension~$\le s$.
%Conversely, 
Any shift-invariant subspace of $\C(\Z)$ of dimension~$s$ is the set of solutions for some homogeneous linear difference equation~$\sP(\Delta) x \equiv 0$ with a characteristic polynomial~$\sP(z) = \sP_0 + \sP_1 z + ... + \sP_s z^s$ of degree~$s$,  unique if normalized by~$\sP(0)=1$.
%\end{enumerate}
\end{proposition}

Recall that for~$w_1, ..., w_s \in \C$, we let~$\X(w_1,...,w_s)$ be the solution set of the equation~\eqref{eq:intro-ODE} whose characteristic polynomial is 
$
\sP(z) = \prod_{k \in [s]} \left(1-{w_k}{z}\right),
$
i.e.~has~$w_1^{-1}, ..., w_s^{-1}$ as its roots. By Proposition~\ref{prop:SIS-characterization}, any SIS of dimension~$s$ writes as~$X(w_1, ..., w_s)$ for a unique, up to a permutation, selection of~$(w_1, ..., w_s) \in \C^s$.
In the case of distinct roots,~$X(w_1, ..., w_s)$ is the span of~$s$ complex exponentials~$w_1^t,..., w_s^t$, i.e.~comprises signals of the form
$x_t = \sum_{k = 1}^s c_k^{\vphantom t} w_k^t$ with~$c_k \in \C.$
Generally, we get exponential polynomials: if the root~$w_{k}^{-1}$ of~$\sP$ has multiplicity~$m_k$, then~$X(w_1, ..., w_s)$ comprises signals of the form~$x_t = \sum_{k \in [s]} q_k(t)^{\vphantom t} w_{k}^t$, where~$\deg(q_k) = m_k-1$ and~$\sum_{k \in [s]} m_k = s$. 

\subsection{Minimal-norm one-sided reproducing filter for the polynomial subspace}
\label{apx:one-sided}

\begin{proposition}
\label{prop:causal-bound}
Let~$X$ be the space of complex polynomials of degree at most~$s-1$. 
Any sequence~$\{\phi_+^{*,m} \in \C_m^{+}(\Z)\}_{m \in \N}$ of one-sided reproducing for~$X$ filters of minimal~$\ell_2$-norm satisfies
\begin{equation}
\label{eq:causal-bound}
\lim_{m \to \infty} m\|\phi_+^{*,m}\|_{2}^2 =  s^2. 
\end{equation}
\end{proposition}
\begin{proof}
%We can w.l.o.g.~assume that~$\phi := \phi^{(m)}$ satisfies~$\phi_0 = 0$. 
%Indeed, assume that we found a reproducing filter~$\phi \in \C_m^+(\Z)$ with~$\phi(0) = 0$ and~$\|\phi\|_2 < s(m+1)^{-1/2}$. Then, 
%Indeed, since~$\|\phi^{(m)}\|_{2} \ge |\phi_0|$, 
%$\lim_{m \to \infty}\sqrt{m+1}\|\phi^{(m)}\|_{2} < s$ is only possible if~$|\phi_0^{(m)}| \to 0$. 
%
%Indeed, if~$\phi(0) \ne 0$, we can consider~$\psi(z) = \phi(z)/\phi(0)$ such that~$\psi(z) = 1$. 
%Let us associate~$\phi = \phi^{(m)}$ with a vector~$asd$
Fixing~$m \ge s$, we first focus on~$\psi \in \C_m^+(\Z)$ such that~$\psi(0) = 0$, denoted as~$\psi \in \C_m^{++}(\Z)$, 
and associate any such~$\psi$ with a vector~$(\psi_1, ..., \psi_m)$. We return to the general case in the end.

\noindent
\proofstep{1}. 
Observe that~$X$ is reproduced by~$\psi \in \C_m^{++}(\Z)$ if and only if~$\psi$ satisfies the equations
\begin{equation}
\label{eq:poly-linsys}
\begin{bmatrix}
1 & 1 & 1 & \dots & 1 \\
0 & \frac{1}{m} & \frac{2}{m} & \dots & 1 \\
%0 & (\frac{1}{m})^2 & (\frac{2}{m})^2 & \dots & 1 \\
\vdots & \vdots & \vdots & \ddots & \vdots \\
0 & \left(\frac{1}{m}\right)^{s-1} & \left(\frac{2}{m} \right)^{s-1} & \dots & 1
\end{bmatrix}
\begin{bmatrix}
-1\\
\psi
%\psi_1\\
%\psi_2\\
%\vdots\\
%\psi_m
\end{bmatrix}
= 0.
\end{equation}
Indeed, each row in~\eqref{eq:poly-linsys} is the slice~$(x_0, x_1, ..., x_m)$ of~$x \in X$, so any reproducing~$\psi \in \C_m^{++}(\Z)$ satisfies~\eqref{eq:poly-linsys}. Conversely, the rows in~\eqref{eq:poly-linsys} slice a monomial basis of~$X$, so any solution to~\eqref{eq:poly-linsys} reproduces an arbitrary~$x \in X$ at~$t = 0$, but then at any~$t \in \Z$ as well, since~$X$ is shift-invariant. 
%there exists~$\wt x \in X:$~$(x_{t}, x_{t+1}, ..., x_{t+m}) = (\wt x_{0}, \wt x_1, ..., \wt x_{m})$ 

\noindent\proofstep{2}. 
Letting~$e_0$ be the first canonical basis vector of~$\R^s$,  we can rewrite~\eqref{eq:poly-linsys} as
\begin{equation}
\label{eq:poly-linsys-resolved}
\begin{bmatrix}
1 & 1 & \dots & 1 \\
\frac{1}{m} & \frac{2}{m} & \dots & 1 \\
%(\frac{1}{m})^2 & (\frac{2}{m})^2 & \dots & 1 \\
\vdots & \vdots & \ddots & \vdots \\
\left(\frac{1}{m}\right)^{s-1} & \left(\frac{2}{m}\right)^{s-1} & \dots & 1
\end{bmatrix}
\psi 
= 
e_0,
%\begin{bmatrix}
%1\\
%0\\ 
%\vdots\\
%0
%\end{bmatrix},
\end{equation}
that is~$V^\top \psi = e_0$ where~$V = {V}_{s}(\frac{1}{m},\frac{2}{m},...,1) \in \R^{m \times s}$ is a full-rank Vandermonde matrix for the interpolation grid~$\{\frac{1}{m}, \frac{2}{m}, ..., 1 \}$.
%for the interpolation grid~$\{\frac{1}{m+1},\frac{2}{m+1},...,\frac{m}{m+1}\}$.
The minimal-norm solution~$\psi^{*,m}_{++}$ of~\eqref{eq:poly-linsys-resolved} is unique and reads
\[
\psi^{*,m}_{+,+} = V (V^\top V)^{-1} e_0,
\]
so that~$m \|\psi^{*,m}_{+,+}\|_2^2 = [H_{s,m}^{-1}]_{0,0}$ where~$H_{s,m} := \frac{1}{m} V^\top V$. 
But for the entries of~$H_{s,m}$ we have
\[
\lim_{m \to \infty} [H_{s,m}]^{\vphantom{m}}_{j,k} 
= \lim_{m \to \infty} \frac{1}{m+1} \sum_{\tau = 1}^m \left(\frac{\tau}{m+1}\right)^{j+k} 
= \int_{0}^{1} u^{j+k} du
= \frac{1}{j+k+1}
= [H_s]_{j,k}
\]
where~$H_{s}$ is the~$s \times s$ Hilbert matrix (recall that~$j,k \in \{0, ..., s-1\}$ by our indexing convention).
Using the identity~$[H_{s}^{-1}]_{0,0} = s^2$, e.g.~\cite{choi1983tricks}, we arrive at the ``strictly one-sided" version of~\eqref{eq:causal-bound}:
\begin{equation}
\label{eq:strict-causal-bound}
\lim_{m \to \infty} m\|\psi^{*,m}_{++}\|_{2}^2 =  s^2.
\end{equation}
\noindent\proofstep{3}. 
Finally, observe that any reproducing for~$X$ filter~$\phi = (\phi_0, \phi_1, ..., \phi_m) \in \C_m^+(\Z)$ with~$\phi_0 \ne 1$ generates a reproducing for~$X$ filter~$\psi = \frac{1}{1-\phi_0} (0, \phi_1, ..., \phi_m) \in \C_m^{++}(\Z)$ whose squared norm is
\[
\|\psi\|_2^2 = \frac{\| \phi \|_2^2 - |\phi_0|^2}{|1-\phi_0|^2}.
\]
Choosing the minimal-norm~$\phi = \phi^{*,m}_{+}$ in the right-hand side, and comparing with~\eqref{eq:strict-causal-bound}, we get
\[
s^2 
= \lim_{m \to \infty} m\big\|\psi^{*,m}_{++}\big\|_2^2 
\le \liminf_{m \to \infty} m \left(\frac{\big\|\phi_+^{*,m}\big\|_2^2 - \big|[\phi_+^{*,m}]_0\big|^2}{\left|1-[\phi_+^{*,m}]_0\right|^2} \right) 
= \liminf_{m \to \infty}  m \left\|\phi_+^{*,m} \right\|_2^2,
\]
where~$\left|[\phi_+^{*,m}]_0\right| \to 0$ by~\eqref{eq:strict-causal-bound}.
Since
$
\|\psi^{*,m}_{++}\|_2 \ge \|\phi_+^{*,m}\|_2,
$
the squeeze theorem implies~\eqref{eq:causal-bound}.
\end{proof}
